# Supplementary material for: Efficient Certified Training and Robustness Verification of Neural ODEs
Source: arXiv:2303.05246 source file (2023-03-09)
Supplement: Supplementary file 1 [file test-appendix.tex]

\section{Test Appendix} \label{app:test-appendix}

This is some test sentence in the appendix.

\begin{figure}[t]
	\centering
	\includegraphics[height=2cm]{example-image-b}
	\caption{Caption of test figure in appendix.}
	\label{fig:appendix}
\end{figure}
